# Supplementary material for: Complex Edge-State Phase Transitions in 1D Topological Laser Arrays
Source: arXiv:1709.00523 source file (2017-09-02)
Supplement: Supplementary file 1 [file Supplemental_Material.pdf]

# Supplementary Materials - Complex Edge-State Phase Transitions in 1D Topological Laser Arrays

Midya Parto,[1] Steffen Wittek,[1] Hossein Hodaei,[1] Gal Harari,[2] Miguel A. Bandres,[2] Jinhan Ren,[1] Mikael C. Rechtsman,[3] Mordechai Segev,[2] Demetrios N. Christodoulides,[1] and Mercedeh Khajavikhan[1]

[1]*CREOL/College of Optics and Photonics, University of Central Florida, Orlando, Florida 32816, USA*
[2]*Department of Physics, Technion, Israel Institute of Technology, Haifa 32000, Israel*
[3]*Department of Physics, The Pennsylvania State University, University Park, Pennsylvania 16802-6300, USA*

The supplementary material is subdivided into four sections. In the first section the emitted spectra by the SSH laser array as expected from numerical solutions of Eqs. (S1.1) of the main text are presented. The theoretical explanation for the frequency upshift in the bulk spectra of the system is provided in section 2. In section 3, the analytical solution corresponding to the field distribution of the edge state in this SSH lattice is derived, and is shown to vary exponentially with the site number. Finally, section 4 presents the details regarding the complex Berry phase discussed in the main text.

## 1. Theoretically predicted spectra emitted by the PT-symmetric SSH laser array

As presented in the Eqs. (3) of the main text, the dynamics of the PT-symmetric SSH laser array can be described by the following rate equations:

$$\begin{aligned}
\frac{dE_n^A}{dt} &= \frac{1}{2}[-\gamma + \sigma(N_n^A - 1)](1 - i\alpha_H)E_n^A + i\kappa_1 E_n^B + i\kappa_2 E_{n-1}^B \\
\frac{dE_n^B}{dt} &= \frac{1}{2}[-\gamma + \sigma(N_n^B - 1)](1 - i\alpha_H)E_n^B + i\kappa_1 E_n^A + i\kappa_2 E_{n+1}^A \\
\frac{dN_n^A}{dt} &= R_A - \frac{N_n^A}{\tau_r} - F(N_n^A - 1)|E_n^A|^2 \\
\frac{dN_n^B}{dt} &= R_B - \frac{N_n^B}{\tau_r} - F(N_n^B - 1)|E_n^B|^2 \,.
\end{aligned} \tag{S1.1}$$

The simulated spectra expected for the three different phases of the PT-symmetric SSH laser array corresponding to Fig. (4) of the main text are presented in Fig. S1. As evident in this figure, phase I involves single edge-mode operation, which lases close to the central frequency $\omega_0$ (Fig. S1 (a)). In phase II, bulk modes of the system will enter the PT-symmetry broken phase, resulting in extra emission lines in the spectra (Fig. S1 (b)). Finally, in phase III all the supermodes (including the edge modes) acquire nonzero gain and loss. This leads to a more involved emission spectra corresponding to those supermodes associated with gain, as shown in Fig. 1 (c). The qualitative behavior of the system as summarized here is consistent with the experimental results of the right panels in Fig. (5).

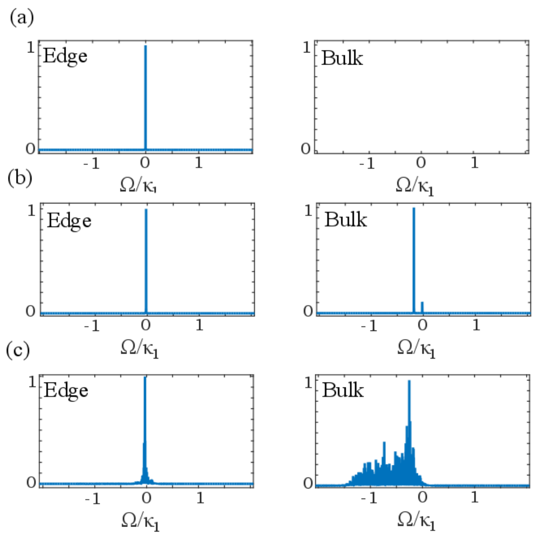


FIG. S1: Calculated spectra for the system considered in Fig. (4) in (a) phase I, (b) phase II, and (c) phase III.

## 2. Frequency upshift in the emission spectra

In this section we present the theoretical analysis which explains the upshift in the frequency spectrum in the PT-symmetric SSH laser array, due to a positive linewidth enhancement factor. In this respect, we consider the modified version of the Hamiltonian of Eq. (4):

$$H_1(k) = \begin{pmatrix} -ig(1-i\alpha_H) & \rho \\ \rho^* & ig(1-i\alpha_H) \end{pmatrix}, \tag{S2.1}$$

where again $\rho = \kappa_1 + \kappa_2 e^{-ik}$, and $\alpha_H$ represents the linewidth enhancement factor. The eigenvalues of this new Hamiltonian can be obtained as:

$$\varepsilon'_{\pm} = \pm\sqrt{|\rho|^2 - g^2(1-i\alpha_H)^2}. \tag{S2.2}$$

For relatively high values of gain which satisfy $|g\alpha_H| \gg |\rho|$, the result of Eq. (S2.2) can be simplified as:

$$\varepsilon'_{\pm} \approx \pm ig(1-i\alpha_H). \tag{S2.3}$$

Now the supermodes which experience gain are the ones associated with $\varepsilon'_{-} \approx -ig - g\alpha_H$, where the negative real part signals an upshift in the resonance frequency for $g, \alpha_H > 0$, due to the chosen base $e^{-i\omega t}$. In other words, in a PT-symmetric active SSH array, the emission spectra of the lasing bulk modes (when the system is operated in phases II and III) will be upshifted with respect to the central frequency $\omega_0$ of the individual rings.

## 3. Analytical solution for the edge mode in the SSH array

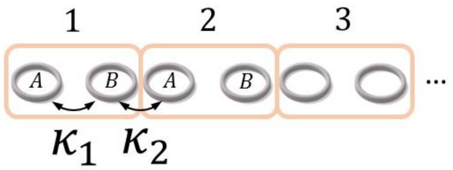


FIG. S2: A schematic of a semi-infinite PT-symmetric SSH microring laser array.

Consider the semi-infinite PT-symmetric SSH array depicted schematically in Fig. S2. The coupled mode equations involving the modal field amplitudes inside the rings are given by:

$$\begin{aligned}\frac{dE_n^A}{dt} &= gE_n^A + i\kappa_1 E_n^B + i\kappa_2 E_{n-1}^B \\ \frac{dE_n^B}{dt} &= -gE_n^B + i\kappa_1 E_n^A + i\kappa_2 E_{n+1}^A ,\end{aligned} \tag{S3.1}$$

with the boundary condition:

$$\frac{dE_1^A}{dt} = gE_1^A + i\kappa_1 E_1^B. \tag{S3.2}$$

We seek solutions of the form $E_n^A = Ae^{iQn}e^{-Pn}e^{\xi t}$ and $E_n^B = Be^{iQn}e^{-Pn}e^{\xi t}$. By direct substitution of these solutions in Eqs. (S3.1-S3.2), one obtains the following solution for the edge state:

$$\begin{aligned}\xi &= g \\ B &= 0 \\ Q &= \pm\pi \\ e^{-P} &= \frac{\kappa_1}{\kappa_2}.\end{aligned} \tag{S3.3}$$

Therefore, the solution for the edge mode in this semi-infinite PT-symmetric SSH array is given by:

$$\begin{aligned}E_n^A &= A\left(-\frac{\kappa_1}{\kappa_2}\right)^n \\ E_n^B &= 0.\end{aligned} \tag{S3.4}$$

## 4. The complex Berry phase for the PT-symmetric SSH Hamiltonian

In general, the Berry phase $\phi$ corresponding to an eigenstate of a non-Hermitian Hamiltonian H(**q**) is given by $\phi = \oint \langle \lambda(\boldsymbol{q}) | \mathrm{i}\nabla_{\boldsymbol{q}} \psi(\boldsymbol{q}) \rangle . d\boldsymbol{q}$ ([1]), where the integral is evaluated on a closed path traced by **q** in the parameter space on which H(**q**) is defined, while $|\psi(\boldsymbol{q})\rangle$ and $|\lambda(\boldsymbol{q})\rangle$ are the right and left (biorthogonal) eigenstates of H(**q**), respectively. From here, the complex Berry phase acquired from the upper (+) and lower (-) bands of the non-Hermitian SSH Hamiltonian can be obtained from the following integral $\phi_\pm = \frac{1}{2}\oint (1 \pm \cos\alpha)\frac{d\theta}{dk}\, dk$ (ref. [31] of main text), where $\alpha = \tan^{-1}\left(\frac{|\rho|}{ig}\right)$ , and $\theta = -\arg(\rho)$. The integration in this equation is performed over the Brillouin zone of the Hamiltonian, i.e. $k \in [-\pi, \pi]$. In the Hermitian limit of $g = 0$, this phase coincides with the conventional Zak phase [2], where $\phi_+ = \phi_- = \phi_Z$ is equal to $\pi$ for $\nu > 1$ and is zero otherwise. This latter equation clearly indicates that the dimerization ratio $\nu = \kappa_2/\kappa_1$ plays an important role in establishing a topological phase transition, a well-known result when dealing with Hermitian SSH arrays. On the other hand, in the presence of non-Hermiticity ($g \neq 0$), the cosine term in the integral will lead to a complex Berry phase. Under these conditions, the geometric phase can be analytically obtained in closed form, and is given by (ref. [31] of main text):

$$\phi_\pm = \phi_h \pm i\frac{\eta}{2}\sqrt{\frac{y}{\nu}}\left(K(y) + \frac{\nu-1}{\nu+1}\Pi(x,y)\right). \tag{S4.1}$$

In this expression the real quantities $x = \frac{4\nu}{(\nu+1)^2}$ , $y = \frac{4\nu}{(\nu+1)^2-\eta^2}$ depend on both the normalized gain $\eta$ and the dimerization coefficient $\nu$, while $K$ and $\Pi$ denote complete elliptic integrals of the first and third

kind, respectively. Figure 4 (d) of main text shows this complex Berry phase associated with the upper band of the Hamiltonian $\phi_+$ as a function of the normalized gain $\eta$ when $\nu = 2$.

## References

[1] J. Garrison and E. Wright, Phys. Lett. A 128, 177 (1988).
[2] J. Zak, Phys. Rev. Lett. 62, 2747 (1989).
